# Supplementary material for: ViLLa: Video Reasoning Segmentation with Large Language Model
Source: arXiv:2407.14500 source file (2025-03-16)
Supplement: Supplementary file 1 [file supp_experiment.tex]

\begin{table*}[t]
    %\vspace{-5pt}
    \centering
    % \caption{\textbf{Comparison on referring video segmentation and video instance segmentation datasets.} }
    \begin{minipage}{0.5\textwidth}
        \centering
        \caption{\textbf{Ablation study} on aggregation strategies.}
        \label{tab:aggregation}
        \scriptsize
        \resizebox{1.0\linewidth}{!}
        {
            \begin{tabular}{l | c c c | c c c}
            \toprule
            \multirow{2}*{Strategy} &  \multicolumn{3}{c |}{Ref-YouTube-VOS} & \multicolumn{3}{c}{Ref-DAVIS17} \\
              & \( \mathcal{J} \)\&\( \mathcal{F} \) & \( \mathcal{J} \) & \( \mathcal{F} \)  &  \( \mathcal{J} \)\&\( \mathcal{F} \) & \( \mathcal{J} \) & \( \mathcal{F} \) \\
            \midrule
            Feature Fusion  &65.9  &64.1  &68.5  &63.2  &60.5  &66.1  \\
            \textbf{Embedding Similarity} &\textbf{66.5}& \textbf{64.6}& \textbf{68.6}&\textbf{64.4} &\textbf{61.2} &\textbf{67.7}\\
            \bottomrule 
            \end{tabular}
        }
            % \end{footnotesize}
    \end{minipage}
    \hfill
    \begin{minipage}{0.48\textwidth}
        \centering        
        \caption{\textbf{Comparison} on VIS datasets (``YTVIS'' refers to ``Youtube-VIS'').}
        \label{tab:vis}
        \vspace{-5pt}
        \resizebox{\linewidth}{!}{
            \tablestyle{12pt}{1.0}
            \begin{tabular}{l|c|c|c}
            \toprule
            \multirow{2}*{Method} &YTVIS-19 &YTVIS-21 &OVIS \\
            &AP &AP &AP\\
            \midrule
            SeqFormer~\cite{wu2022seqformer} &59.3 &51.8 &- \\
            Mask2Former~\cite{cheng2021mask2former} &61.6 &55.3 &24.1 \\
            VITA~\cite{heo2022vita} &63.0 &57.5 &27.7 \\
            IDOL~\cite{wu2022defense} &64.3 &56.1 &42.6 \\
            \cellcolor[HTML]{efefef}{\textbf{ViLLa}} &\cellcolor[HTML]{efefef}\textbf{67.6} &\cellcolor[HTML]{efefef}\textbf{59.9} &\cellcolor[HTML]{efefef}\textbf{46.5} \\
            \bottomrule
            \end{tabular}
        }
    \end{minipage}
    \vspace{-12pt}
\end{table*}
